# Supplementary material for: Cavity-waveguide interplay in lossy resonators and its role in optimal single-photon sources
Source: arXiv:1804.01364 source file (2018-06-13)
Supplement: Supplementary file 1 [file SuppMat_EVD4.pdf]

# Fundamental cavity–waveguide interplay in cavity QED
# Supplemental Information

Emil V. Denning,[1] Jake Iles-Smith,[1] Andreas D. Østerkryger,[1] Niels Gregersen,[1] and Jesper Mørk[1]
[1]*Department of Photonics Engineering, DTU Fotonik, Technical University of Denmark, Building 343, 2800 Kongens Lyngby, Denmark*
(Dated: June 13, 2018)

Here we provide details and derivations of the expressions used in the main text.

## I. SEPARATION OF LOCAL DENSITY OF STATES INTO CAVITY AND WAVEGUIDE PARTS

Here we show in detail, how the local density of states (LDOS) can be separated into a Lorentzian cavity contribution and a spectrally flat waveguide contribution. From Eq. (2) in the main text, we define the dimensionless LDOS,

$$\ell(\omega) = \frac{\mathcal{L}_{\mathcal{B}}(\omega)}{\Gamma^0_{\mathcal{B}}} = \mathrm{Re}\left[\frac{[1+\tilde{r}_1(\omega)][1+\tilde{r}_2(\omega)]}{1-\tilde{r}_1(\omega)\tilde{r}_2(\omega)}\right], \tag{1}$$

where $\tilde{r}_j(\omega) = r_j e^{i[\phi_0^j + L\beta(\omega)]}$ is an effective complex reflectivity coefficient accounting for the propagation phase in the cavity. Here $\phi_0^j$ is the mirror reflection phase, $L$ is the cavity length and $\beta(\omega)$ is the propagation factor, which we take dispersionless, $\beta(\omega) = n_{\mathrm{eff}}\omega/c$, where $n_{\mathrm{eff}}$ is the effective refractive index of the waveguide mode. For convenience, we also define the dimensionless frequency, $\tilde{\omega} = Ln_{\mathrm{eff}}\omega/c$, where the mirror reflection phases have been ignored. We thus have $\tilde{r}_i(\tilde{\omega}) = r_i e^{i\tilde{\omega}}$.

### A. Symmetric cavity

Taking the two mirrors identical, we write $r_1 = r_2 \equiv r$, and the dimensionless LDOS becomes

$$\ell(\tilde{\omega}) = \mathrm{Re}\left[\frac{[1+\tilde{r}(\tilde{\omega})]^2}{1-\tilde{r}(\tilde{\omega})^2}\right] = \frac{1-r^2}{1+r^2-2r\cos\tilde{\omega}}, \tag{2}$$

We now assume that the LDOS contains two contributions: A constant (spectrally flat) background contribution from the waveguide nature of the system and a Lorentzian contribution from the cavity. In the limit $r \to 0$, the constant background is completely dominating, whereas the cavity becomes the only contribution in the limit $r \to 1$. We define this LDOS as

$$\bar{\ell}(\tilde{\omega}) = \ell_{\mathcal{B}} + \ell_c \frac{\tilde{\kappa}}{\tilde{\kappa}^2 + \tilde{\omega}^2}, \tag{3}$$

where $\ell_{\mathcal{B}}$ and $\ell_c$ are the weight of the residual waveguide modes and cavity mode, respectively, and $\tilde{\kappa} = Ln_{\mathrm{eff}}\kappa/c$ is a dimensionless cavity linewidth. To establish a relation between $r$ and $\{\ell_{\mathcal{B}}, \ell_c, \tilde{\kappa}\}$, we now require that three similarity requirements between $\ell$ and $\bar{\ell}$ are fulfilled: 1) The values of $\ell$ and $\bar{\ell}$ at $\tilde{\omega} = 0$ should be equal, 2) the second derivatives of $\ell$ and $\bar{\ell}$ at $\tilde{\omega} = 0$ should be equal and 3) the integral of $\ell$ and $\bar{\ell}$ over the range $[-\pi, \pi]$ should be equal. The first requirement leads to the equation

$$\bar{\ell}(0) = \ell(0) \Rightarrow \ell_{\mathcal{B}} + \frac{\ell_c}{\tilde{\kappa}} = \frac{1-r^2}{(1-r)^2}. \tag{4}$$

The second requirement amounts to

$$\frac{\mathrm{d}^2}{\mathrm{d}\tilde{\omega}^2}\bar{\ell}(0) = \frac{\mathrm{d}^2}{\mathrm{d}\tilde{\omega}^2}\ell(0) \Rightarrow \ell_c = \frac{r(1-r^2)}{(1-r)^4}\tilde{\kappa}^3. \tag{5}$$

The third requirement is more involved and reads

$$\int_{-\pi}^{\pi} \mathrm{d}\tilde{\omega}\,\bar{\ell}(\tilde{\omega}) = \int_{-\pi}^{\pi} \mathrm{d}\tilde{\omega}\,\ell(\tilde{\omega}) \\ \Rightarrow \pi\ell_{\mathcal{B}} + \ell_c \arctan(\pi/\tilde{\kappa}) = \pi. \tag{6}$$

Inserting (5) into (4) yields

$$\ell_{\mathcal{B}} = \frac{1-r^2}{(1-r)^2}\left[1 - \frac{r\tilde{\kappa}^2}{(1-r)^2}\right]. \tag{7}$$

Inserting this into (6), we obtain the implicit equation

$$\frac{1}{\pi}\tilde{\kappa}^3 \arctan(\pi/\tilde{\kappa}) - \tilde{\kappa}^2 = \frac{(1-r)^2}{r}\left[\frac{(1-r)^2}{1-r^2} - 1\right]. \tag{8}$$

Given a particular value of the parameter $r$, this equation can be solved for $\tilde{\kappa}$ numerically with a unique value. When $\tilde{\kappa}$ is found, $\ell_{\mathcal{B}}$ and $\ell_c$ can be calculated using (5) and (7). We can relate the emitter–cavity coupling rate, $g$, to the parameters $\{\ell_c, \Gamma^0_{\mathcal{B}}\}$ using the well-known result $\Gamma_{\mathrm{cav}} = 4g^2/\kappa$ for the resonant cavity-enhanced spontaneous emission rate [1], which must correspond to the cavity contribution to the LDOS. The spontaneous emission rate on resonance calculated through (3) is

$$\Gamma^0_{\mathcal{B}}\bar{\ell}(0) = \Gamma^0_{\mathcal{B}}\ell_{\mathcal{B}} + \frac{\Gamma^0_{\mathcal{B}}\ell_c}{\tilde{\kappa}}. \tag{9}$$

From this, we identify the cavity contribution $\Gamma_{\mathrm{cav}} = \Gamma^0_{\mathcal{B}}\ell_c/\tilde{\kappa}$, leading to

$$g = \sqrt{\frac{\Gamma^0_{\mathcal{B}}\ell_c c}{4Ln_{\mathrm{eff}}}}. \tag{10}$$

### B. Perfect bottom mirror

Here we consider a more practical situation, where one of the cavity mirrors is perfectly reflecting, $r_1 = 1, r_2 \equiv r$. The LDOS then becomes

$$\ell(\tilde{\omega}) = \mathrm{Re}\left[\frac{(1+e^{i\tilde{\omega}})(1+re^{i\tilde{\omega}})}{1-re^{2i\tilde{\omega}}}\right] = \frac{(1-r^2)(1+\cos\tilde{\omega})}{1+r^2-2r\cos 2\tilde{\omega}} = \frac{1-r^2}{1+r^2-2r\cos 2\tilde{\omega}} + \frac{(1-r^2)\cos\tilde{\omega}}{1+r^2-2r\cos 2\tilde{\omega}}. \tag{11}$$

The first term of this expression is very similar to the symmetric-cavity LDOS, but the second one does not become frequency independent in the limit $r = 0$, but rather describes an oscillation with period $2\pi$. This oscillation is due to interference between the directly transmitted light and the reflected light from the bottom mirror [2]. However, the oscillation period with respect to $\omega$ is $2\pi c/(Ln_{\mathrm{eff}})$, which for a $\lambda$-cavity is twice the emitter transition frequency, typically corresponding to hundreds of meV. Thus, we Taylor expand $\cos\tilde{\omega}$ around $\tilde{\omega} = 0$, keeping only the zeroth order term, which is unity. The LDOS then becomes

$$\ell(\tilde{\omega}) \simeq \frac{2(1-r^2)}{1+r^2-2\cos 2r\tilde{\omega}} \tag{12}$$

This is equal to the LDOS for a symmetric cavity, (2), besides from an overall factor of 2 and the substitution $\tilde{\omega} \to \tilde{\omega}/2$. Thus, we can determine the parameters $\ell_{\mathcal{B}}, \ell_c$ and $\tilde{\kappa}$ as described in Sec. I A and subsequently make the substitutions $\ell_{\mathcal{B}} \to 2\ell_{\mathcal{B}}$, $\ell_c \to 2\ell_c$, $\tilde{\kappa} \to \tilde{\kappa}/2$.

### C. Optical master equation

We now write down a Hamiltonian describing the quantum dynamics of the emitter and local electric field. We assume that the emitter can be described as a two level system with ground and excited states, $|g\rangle$ and $|e\rangle$, respectively, separated by the transition energy, $\omega_X$ and with dipole operator $\sigma = |g\rangle\langle e|$. The continuum of optical modes corresponding to the waveguide contribution to the LDOS is described by a set of annihilation (creation) operators, $w_k$ ($w_k^\dagger$), with emitter coupling rates $h_k$ and frequencies $W_k$. The cavity mode is described by a single annihilation (creation) operator, $\hat{a}$ ($\hat{a}^\dagger$) with frequency $\omega_c$. Loss through the cavity mirrors is captured by coupling of the cavity to a set of optical modes with annihilation (creation) operators $v_k$ ($v_k^\dagger$), frequencies $V_k$, and cavity coupling rates $f_k$. Finally, the emitter also couples to other optical modes than the mode set of interest. These modes are described by a set of annihilation (creation) operators $p_k$ ($p_k^\dagger$) with frequencies $P_k$ and emitter coupling rates $d_k$. The Hamiltonian describing these interactions is $H = H_{\mathrm{S}} + H_{\mathrm{F}} + H_{\mathrm{SF}}$, where $H_{\mathrm{S}}$ describes the emitter–cavity system, $H_{\mathrm{F}}$ describes the non-cavity modes of the electric field, $H_{\mathrm{SF}}$ describes the interaction between the emitter–cavity system and the non-cavity modes. They take the standard forms

$$\begin{aligned} H_{\mathrm{S}} &= \omega_X |e\rangle\langle e| + \omega_c \hat{a}^\dagger\hat{a} + g(\sigma^\dagger\hat{a} + \sigma\hat{a}^\dagger), \\ H_{\mathrm{F}} &= \sum_k W_k w_k^\dagger w_k + \sum_k V_k v_k^\dagger v_k + \sum_k P_k p_k^\dagger p_k, \\ H_{\mathrm{SF}} &= \sum_k h_k \sigma^\dagger w_k + \sum_k f_k \hat{a}^\dagger v_k + \sum_k d_k \sigma^\dagger w_k + \mathrm{H.c.}. \end{aligned} \tag{13}$$

We treat the non–cavity modes perturbatively by deriving a Born-Markov master equation, where $H_{\mathrm{SF}}$ is treated to second order. This master equation takes the form

$$\dot{\rho}(t) = -i[H_{\mathrm{S}}, \rho(t)] - \int_0^\infty \mathrm{d}\tau\, \mathrm{Tr}_{\mathrm{F}}[H_{\mathrm{F}}, [\tilde{H}_{\mathrm{F}}(-\tau), \rho(t)\otimes F_0]], \tag{14}$$

where $\rho$ is the density operator for the emitter–cavity system, $\mathrm{Tr}_F$ denotes a trace over the field Hilbert space, $\tilde{H}_{SF}(t) = e^{i[H_{\mathrm{F}}+H_{\mathrm{S}}]t} H_{\mathrm{SF}} e^{-i[H_{\mathrm{F}}+H_{\mathrm{S}}]t}$ is the system–field Hamiltonian in the interaction picture and $F_0 = e^{-H_{\mathrm{F}}/(k_B T)} / \mathrm{Tr}\left(e^{-H_{\mathrm{F}}/(k_B T)}\right)$ is the thermal state of the free field (with $k_B$ and $T$ the Boltzmann constant and temperature), approximated as vacuum. Using (13), we obtain the master equation

$$\dot{\rho}(t) = -i[H_{\mathrm{S}}, \rho(t)] + (\Gamma_{\mathcal{B}} + \Gamma_{\mathcal{R}})\mathcal{D}[\sigma] + \kappa\mathcal{D}[\hat{a}], \tag{15}$$

with $\Gamma_{\mathcal{B}} = \pi\sum_k |h_k|^2 \delta(\omega_X - W_k)$, $\Gamma_{\mathcal{R}} = \pi\sum_k |d_k|^2 \delta(\omega_X - P_k)$, $\kappa = \pi\sum_k |f_k|^2 \delta(\omega_c - V_k)$ and $\mathcal{D}[x] = x\rho x^\dagger - \{x^\dagger x, \rho\}$.

## II. EMITTED ELECTRIC FIELD AND OPTICAL GREEN'S FUNCTION

In this section, we calculate the electric field generated by a radiating dipole using a modal method formulation [3]. Here, the structure under consideration is divided into sections featuring translational symmetry along a propagation axis usually chosen as the $z$ axis. The eigenmodes $\mathbf{E}_j^q$, $j = 1, 2, \cdots$ for the $q$'th section are computed under the assumption of uniformity along $z$. The electric field in each section is then expanded on the eigenmodes of the particular section, and the fields in the various sections are connected using a scattering matrix formalism [3].

Inside the cavity section, the forward propagating part of the field above the emitter is expanded on the cavity section eigenmodes $\mathbf{E}_j^C$ as

$$\mathbf{E}(\mathbf{r},\omega) = \sum_j a_j^C(\omega)\mathbf{E}_j^C(\mathbf{r}_\perp,\omega)e^{i\beta_j(z-z_0)}, \quad (z_0 \le z \le z_2) \tag{16}$$

where $a_j^C$ are the modal expansion coefficients for the cavity section and $z_0$ ($z_2$) is the $z$ coordinate of the

emitter (top mirror). In the case of an infinite waveguide ($r_1 = r_2 = 0$), the modal expansion coefficients are $a_j^{C\infty}(\omega) = i\omega\mathbf{p}(\omega)\cdot\mathbf{E}_j^C(\mathbf{r}_\perp^0,\omega)/2$, where $\mathbf{p}$ is the dipole moment of the emitter positioned at $(\mathbf{r}_\perp^0, z_0)$. In this notation, $a_1^{C\infty}(\omega) = a_{\mathcal{B}}^{C\infty}(\omega)$ is the expansion coefficient for the fundamental guided mode $\mathbf{E}_1^C = \mathbf{E}_{\mathcal{B}}^C$ and $a_j^{C\infty}(\omega)$ for $j > 1$ describe contributions to the set $\mathcal{R}$ of other guided modes and radiation modes.

We now assume that the device and the experimental setup are optimized for a single transverse mode $\mathcal{B}$, such that all other modes are lost or filtered out. When taking the cavity mirrors into account and assuming a dipole oriented in the $x-y$ plane, we then find the corresponding expansion coefficient $a_{\mathcal{B}}^C$ for the forward propagating mode $\mathbf{E}_{\mathcal{B}}^C$ in the cavity region as [3]

$$a_{\mathcal{B}}^C(\omega) = \frac{1+\tilde{r}_1(\omega)}{1-\tilde{r}_1(\omega)\tilde{r}_2(\omega)} a_{\mathcal{B}}^{C\infty}(\omega). \tag{17}$$

In the waveguide region on the right side of mirror 2, the modal structure is given by the same transverse modes $\mathbf{E}_j^W \equiv \mathbf{E}_j^C \equiv \mathbf{E}_j$ as inside the cavity region with an expansion similar to (16). Here, the expansion coefficient $a_{\mathcal{B}}^W$ for $\mathcal{B}$ is given by $a_{\mathcal{B}}^W = \tilde{t}_2(\omega)a_{\mathcal{B}}^C$, where $\tilde{t}_2(\omega) = t_2 e^{i[\theta_2+\beta(\omega)L/2]}$ accounts for propagation from the emitter to mirror 2 and subsequent transmission through mirror 2 and $\theta_2$ is a mirror transmission phase.

The detected electric field operator for the field outside the cavity ($z_2 \le z$) then becomes

$$\mathbf{E}(\mathbf{r},\omega) = \frac{i\omega}{2}\mathcal{G}(\omega)e^{i\beta(\omega)[z-z_2]}\mathbf{E}_{\mathcal{B}}(\mathbf{r}_\perp,\omega)\otimes\mathbf{E}_{\mathcal{B}}(\mathbf{r}_\perp^0,\omega)\cdot\mathbf{p}, \tag{18}$$

where $\mathcal{G}(\omega) = \tilde{t}_2[1+\tilde{r}_1(\omega)][1-\tilde{r}_1(\omega)\tilde{r}_2(\omega)]^{-1}$.

As for the power $P_{\mathcal{B}}$ emitted through mirror 2, we use Poyntings theorem to find

$$P_{\mathcal{B}}(\omega) = \int \mathrm{d}\mathbf{r}_\perp \,\mathrm{Re}[\mathbf{E}(\mathbf{r},\omega)\times\mathbf{H}(\mathbf{r},\omega)]\cdot\mathbf{e_z} = \frac{1}{2}|\mathcal{G}(\omega)|^2 P_{\mathcal{B}}^0(\omega), \tag{19}$$

where $P_{\mathcal{B}}^0(\omega)$ is the power emitted by the dipole into the mode set $\mathcal{B}$ in the absence of cavity mirrors. This can simply be described as emission into a frequency independent reservoir with spontaneous emission rate $\Gamma_{\mathcal{B}}^0$. Relative to emission in a bulk medium, we have $P_{\mathcal{B}}^0(\omega)/P_{\mathrm{bulk}}(\omega) = \Gamma_{\mathcal{B}}^0(\omega)/\Gamma_{\mathrm{bulk}}(\omega)$, where $P_{\mathrm{bulk}}$, $\Gamma_{\mathrm{bulk}}$ are the emitted power and spontaneous emission rate into a bulk medium, respectively [4]. Similarly, the emitted power into the radiative reservoir, $\mathcal{R}$, is $P_{\mathcal{R}}(\omega)/P_{\mathrm{bulk}}(\omega) = \Gamma_{\mathcal{R}}(\omega)/\Gamma_{\mathrm{bulk}}(\omega)$.

## III. POLARON MASTER EQUATION

Taking longitudinal acoustic phonons into account, the Hamiltonian becomes $H = H_{\mathrm{S}} + H_{\mathrm{F}} + H_{\mathrm{P}} + H_{\mathrm{SF}} + H_{\mathrm{SP}}$, where $H_{\mathrm{S}}$, $H_{\mathrm{F}}$ and $H_{\mathrm{SF}}$ are given by (13) and the free phonon and system–phonon interaction Hamiltonians are [5, 6]

$$H_{\mathrm{P}} = \sum_{\mathbf{q}} \nu_{\mathbf{q}} b_{\mathbf{q}}^\dagger b_{\mathbf{q}}, \tag{20}$$

$$H_{\mathrm{SP}} = |e\rangle\langle e| \sum_{\mathbf{q}} M_{\mathbf{q}}(b_{\mathbf{q}} + b_{\mathbf{q}}^\dagger), \tag{21}$$

where the phonon mode with wavevector $\mathbf{q}$, frequency $\nu_{\mathbf{q}}$ and emitter coupling rate $M_{\mathbf{q}}$ is described by a bosonic annihilation (creation) operator $b_{\mathbf{q}}$ ($b_{\mathbf{q}}^\dagger$). The phonon modes are described by the spectral density $\mathcal{J}(\nu) = \sum_{\mathbf{q}} M_{\mathbf{q}}^2\delta(\nu-\nu_{\mathbf{q}}) = \alpha\nu^3 e^{-\nu^2/\nu_c^2}$, where $\nu_c$ is the phonon cutoff frequency and $\alpha$ is the electron–phonon coupling strength [7]. Before deriving the master equation as in Sec. I C, we first apply the unitary polaron transformation, $\mathcal{T} = |0\rangle\langle 0| + |X\rangle\langle X|\,B_+$, with $B_\pm = \exp\Big[\pm\sum_{\mathbf{q}}\frac{M_{\mathbf{q}}^2}{\nu_{\mathbf{q}}}(b_{\mathbf{q}}^\dagger - b_{\mathbf{q}})\Big]$, to account for non-Markovian exciton–phonon dynamics [7–11]. The polaron-transformed Hamiltonian is $\hat{H} = \mathcal{T}H\mathcal{T}^\dagger = \hat{H}_{\mathrm{S}} + \hat{H}_{\mathrm{F}} + \hat{H}_{\mathrm{P}} + \hat{H}_{\mathrm{I}}$, where $\hat{H}_{\mathrm{F}} = H_{\mathrm{F}}$, $\hat{H}_{\mathrm{P}} = H_{\mathrm{P}}$ and

$$\begin{aligned} \hat{H}_{\mathrm{S}} &= (\omega_X - \epsilon)\,|e\rangle\langle e| + \omega_c\hat{a}^\dagger\hat{a} + gB\hat{e} \\ \hat{H}_{\mathrm{I}} &= g(\hat{X}B_X + \hat{Y}B_Y) + \sum_k h_k\sigma^\dagger B_+ w_k \\ &\quad + \sum_k d_k\sigma^\dagger B_+ p_k + \sum_k f_k\hat{a}^\dagger v_k + \mathrm{H.c.}, \end{aligned} \tag{22}$$

where $\hat{X} = \sigma^\dagger\hat{a} + \sigma^\dagger\hat{a}$, $\hat{Y} = i(\sigma^\dagger\hat{a} - \sigma\hat{a}^\dagger)$, $B_X = (B_+ + B_- - 2)/2$, $B_Y = i(B_+ - B_-)/2$, $B = Tr[B_\pm e^{-H_{\mathrm{P}}/(k_BT)}]/Tr[e^{-H_{\mathrm{P}}/(k_BT)}]$ and $\epsilon = 2\sum_{\mathbf{q}} M_{\mathbf{q}}^2/\nu_{\mathbf{q}}$ is a phonon induced renormalisation of the emitter transition energy, which we absorb into $\omega_X$. In this frame, we derive a Born-Markov master equation, where $\hat{H}_{\mathrm{I}}$ is treated perturbatively to second order, similar to (14),

$$\begin{aligned} \frac{\mathrm{d}}{\mathrm{d}t}\rho(t) &= -i[H_{\mathrm{S}}, \rho(t)] \\ &\quad - \int_0^\infty \mathrm{d}\tau\,\mathrm{Tr}_{\mathrm{F,P}}[H_{\mathrm{I}}, [\tilde{H}_{\mathrm{I}}(-\tau), \rho(t)\otimes F_0\otimes P_0]], \end{aligned} \tag{23}$$

where the trace is now performed over the Hilbert spaces of both the electric field and phonons, and $P_0 = e^{-\hat{H}_{\mathrm{P}}/(k_BT)}/\,\mathrm{Tr}\left(e^{-\hat{H}_{\mathrm{P}}/(k_BT)}\right)$ is the thermal state of the phonons. The caret over the density operator signifies that is calculated in the polaron frame. This master equation reduces to

$$\begin{aligned} \frac{\mathrm{d}}{\mathrm{d}t}\rho(t) &= -i[\hat{H}_{\mathrm{S}}, \rho(t)] + (\Gamma_{\mathcal{B}} + \Gamma_{\mathcal{R}})\mathcal{D}[\sigma] \\ &\quad + \kappa\mathcal{D}[\hat{a}] + \mathcal{K}_{\mathrm{P}}[\rho(t)], \end{aligned} \tag{24}$$

where

$$\mathcal{K}_{\mathrm{P}}[\rho] = -g^2\Big\{\gamma_X[\hat{X},\hat{X}\rho] + \gamma_Y[\hat{Y},\hat{Y}\rho] + \gamma_Z[\hat{Y},\hat{Z}\rho] + \mathrm{H.c.}\Big\}, \tag{25}$$

where $\hat{Z} = \sigma^\dagger\sigma - \hat{a}^\dagger\hat{a}$ and $\gamma_X = \int_0^\infty \mathrm{d}\tau\, \Lambda_X(\tau)$, $\gamma_Y = \int_0^\infty \mathrm{d}\tau \cos[2gB\tau]\Lambda_Y(\tau)$, $\gamma_Z = -\int_0^\infty \mathrm{d}\tau \sin[2gB\tau]\Lambda_Y(\tau)$. The free phonon correlation functions $\Lambda_{X,Y}$ are given by $\Lambda_X(\tau) = \left\langle \tilde{B}_X(\tau)B_X \right\rangle = B^2(e^{\phi}(\tau) + e^{-\phi(\tau)} - 2)/2$, $\Lambda_Y(\tau) = B^2(e^{\phi(\tau)} - e^{-\phi(\tau)})/2$, where $\phi(\tau) = \int_0^\infty \mathrm{d}\nu\, \mathcal{J}(\nu)/\nu^2\{\coth[\nu/(2k_BT)]\cos(\nu\tau) - i\sin(\nu\tau)\}$. Any additional pure dephasing noise with a rate $\gamma$ can be included in the master equation by adding the term $2\gamma\mathcal{D}[\sigma^\dagger\sigma]$ to the RHS of (24) [12]

Importantly, when calculating expectation values and two-time correlation functions using the master equation, we need to apply the inverse polaron transformation, or transform the operators of interest to the polaron frame as well. For the dipole two-time correlation function, this is carried out as

$$\langle\sigma^\dagger(t)\sigma(t')\rangle = \mathrm{Tr}[\zeta^\dagger(t)\zeta(t')\hat{\chi}(0)], \tag{26}$$

where $\zeta = \mathcal{T}\sigma\mathcal{T}^\dagger = B_-\sigma$ and $\hat{\chi}$ is the density operator of the composite emitter–phonon Hilbert space in the polaron frame. By taking the phonon and emitter uncorrelated in the polaron frame, we can write $\mathrm{Tr}\left[\sigma^\dagger(t)B_+(t)B_-(t')\sigma(t')\hat{\chi}(0)\right] \simeq \mathrm{Tr}[B_+(t)B_-(t')P_0]\,\mathrm{Tr}\left[\sigma^\dagger(t)\sigma(t')\hat{\rho(0)}\right]$, where the free phonon correlation function is $\mathrm{Tr}[B_+(t)B_-(t')P_0] = B^2e^{\phi(t-t')}$.

The indistinguishability is calculated through the coherence function of the electric field [13],

$$\mathcal{I} = \frac{\int \mathrm{d}\mathbf{r}_\perp \int_{-\infty}^{\infty}\mathrm{d}t \int_{-\infty}^{\infty}\mathrm{d}\tau\, \left|\langle\mathbf{E}^\dagger_{\mathcal{B}}(\mathbf{r},t+\tau)\mathbf{E}_{\mathcal{B}}(\mathbf{r},t)\rangle\right|^2}{\int \mathrm{d}\mathbf{r}_\perp \left[\int_{-\infty}^{\infty}\mathrm{d}t\, \langle\mathbf{E}^\dagger_{\mathcal{B}}(\mathbf{r},t)\mathbf{E}_{\mathcal{B}}(\mathbf{r},t)\rangle\right]^2}. \tag{27}$$

Using (18), where we assume that the transverse mode profile of the electric field does not vary appreciably as a function of frequency over the range of interest, $\mathbf{E}_{\mathcal{B}}(\mathbf{r}_\perp,\omega) \simeq \mathbf{E}_{\mathcal{B}}(\mathbf{r}_\perp,\omega_X)$, this becomes [11]

$$[2\mathcal{P}_{\mathcal{B}}/\Gamma^0_{\mathcal{B}}]^{-2}\int \mathrm{d}\omega\, \left|\mathcal{G}^*(\omega)\mathcal{G}(\omega')\,\langle\sigma^\dagger(\omega)\sigma(\omega')\rangle\right|^2, \tag{28}$$

where $\sigma(\omega) = \int \mathrm{d}t\, \sigma(t)e^{-i\omega t}$ and $\mathcal{P}_{\mathcal{B}} = (\Gamma^0_{\mathcal{B}}/2)\int_{-\infty}^{\infty}\mathrm{d}\omega\, |\mathcal{G}(\omega)|^2 S_0(\omega,\omega)$.

The efficiency is calculated as the ratio of power in the desired radiation channel, $\mathcal{B}$, and the total emission, i.e. into both sets $\mathcal{B}$ and $\mathcal{R}$,

$$\mathcal{E} = \frac{\int_{-\infty}^{\infty}\mathrm{d}\omega\, P_{\mathcal{B}}(\omega)}{\int_{-\infty}^{\infty}\mathrm{d}\omega\, [P_{\mathcal{B}}(\omega) + P_{\mathcal{R}}(\omega)]} = \frac{\mathcal{P}_{\mathcal{B}}}{\mathcal{P}_{\mathcal{B}} + \mathcal{P}_{\mathcal{R}}}, \tag{29}$$

where $\mathcal{P}_{\mathcal{R}} = \Gamma_{\mathcal{R}}\int_{-\infty}^{\infty}\mathrm{d}\omega\, S_0(\omega,\omega)$.


[1] H. J. Carmichael, *Statistical Methods in Quantum Optics 1: Master Equations and Fokker-Planck Equations* (Springer Science & Business Media, 2009).

[2] N. Gregersen, D. P. McCutcheon, J. Mørk, J.-M. Gérard, and J. Claudon, Optics express **24**, 20904 (2016).

[3] A. V. Lavrinenko, J. Lægsgaard, N. Gregersen, F. Schmidt, and T. Søndergaard, *Numerical methods in photonics*, Vol. 1 (CRC Press, 2014).

[4] L. Novotny and B. Hecht, *Principles of nano-optics* (Cambridge university press, 2012).

[5] G. D. Mahan, *Many-particle physics* (Springer Science & Business Media, 2013).

[6] A. Ramsay, T. Godden, S. Boyle, E. M. Gauger, A. Nazir, B. W. Lovett, A. Fox, and M. Skolnick, Physical Review Letters **105**, 177402 (2010).

[7] A. Nazir and D. P. McCutcheon, Journal of Physics: Condensed Matter **28**, 103002 (2016).

[8] D. P. McCutcheon and A. Nazir, New Journal of Physics **12**, 113042 (2010).

[9] C. Roy and S. Hughes, Physical Review X **1**, 021009 (2011).

[10] I. Wilson-Rae and A. Imamoğlu, Physical Review B **65**, 235311 (2002).

[11] J. Iles-Smith, D. P. McCutcheon, A. Nazir, and J. Mørk, Nature Photonics **11**, 521 (2017).

[12] T. Grange, N. Somaschi, C. Antón, L. De Santis, G. Coppola, V. Giesz, A. Lemaître, I. Sagnes, A. Auffèves, and P. Senellart, Physical Review Letters **118**, 253602 (2017).

[13] A. Kiraz, M. Atatüre, and A. Imamoğlu, Physical Review A **69**, 032305 (2004).
